# Supplementary material for: DDL-MVS: Depth Discontinuity Learning for MVS Networks
Source: arXiv:2203.01391 source file (2023-06-12)
Supplement: Supplementary file 1 [file supp.tex]

\paragraph{ Difference with SMDNets (two-view stereo) \cite{Tosi2021CVPR}.}
To the best of our knowledge, our work is the first learning-based MVS method that explicitly learns depth discontinuity maps (aka geometric edge maps) to simultaneously refine the quality and improve the smoothness of the depth maps. 
Different from SMD-Nets, we use the UNet shape 2DCNN architecture instead of the MLP, which makes our pipeline efficient in terms of time and memory consumption. 
Besides extending bimodal depth estimation to the multi-view case, our work also shows that with a single refinement auto-encoder, it is possible to achieve three goals: (1) Upsampling; (2) Refining; (3) Multi-task learning. We use the same single auto-encoder to regress both bimodal distribution parameters and boundary maps. 
Our 
During the training, we logged the depth map error of PatchMatch Stereo, from which we observed that the depth map error was reduced from 7.09 $mm$ to 5.28 $mm$ with the refinement network. This quantitative measure shows that our refinement module improves the depth map quality by reducing the error roughly by $25 \%$. 

%===========================================================
\paragraph{ Comparison with the classical method using Gipuma Fusion.}
While carrying out the experiment reported in Table 1, we used the same fusion pipeline with the same fusion parameters as in the baseline method. In the paper, we use the same fusion pipeline that MVSNet\cite{yao_2018_mvsnet} and our baseline use. To show the fair advantage of our work over the traditional MVS, we have tried to run \textbf{default} Gipuma\cite{galliani_2015_gipuma} fusion without any hyperparameter and filter tuning. The evaluation was carried out using the benchmark in Table 1, and the results are shown in the table below, from which we can see that our method is superior in terms of all three metrics. Certainly, the overall metric can be further improved with proper parameter tuning.
\begin{center}
	\begin{tabular}{||c c c c||} 
		\hline
		Method & Acc & Comp & Overall \\ [0.5ex] 
		\hline\hline
		Gipuma [27] & 0.283 & 0.873 & 0.578 \\
		Ours ($L_{1,2,3,4}$)&  \textbf{0.270}  &  \textbf{0.776} & \textbf{ 0.523}\\\hline
	\end{tabular}
\end{center}
%===========================================================
%===========================================================
%===========================================================

%===========================================================

%===========================================================
\paragraph{Why is the learned edge map better?}
In the earlier stage of the development of DDL-MVS, we tried to feed the network with HED\cite{xie2015holistically} output and jointly refine the depth and edge maps similar to EdgeStereo\cite{song2018edgestereo}. It turned out that even after refinement, the edges were too sensitive to photometric changes (shadows, variations in illumination and color, small changes in depth), leading to higher depth errors.
%===========================================================

\begin{figure}[!hp]
	\advance\leftskip-0.14cm
	\begin{tabular}{c@{}c@{}c@{}c}
		\includegraphics[width=0.235\linewidth]{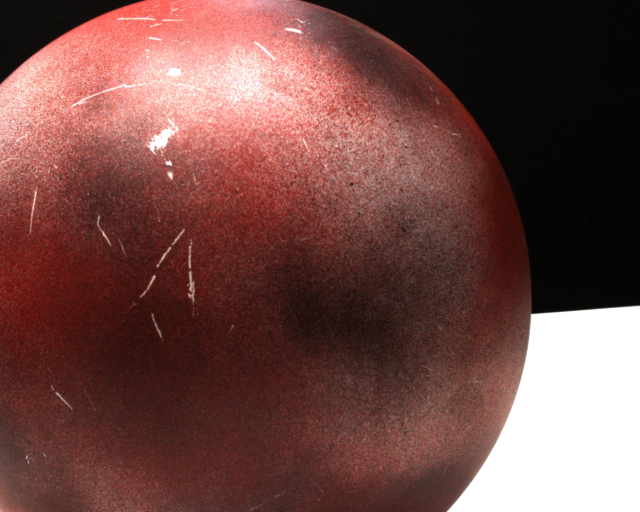}&
		\hspace{0.1cm}
		\includegraphics[width=0.235\linewidth]{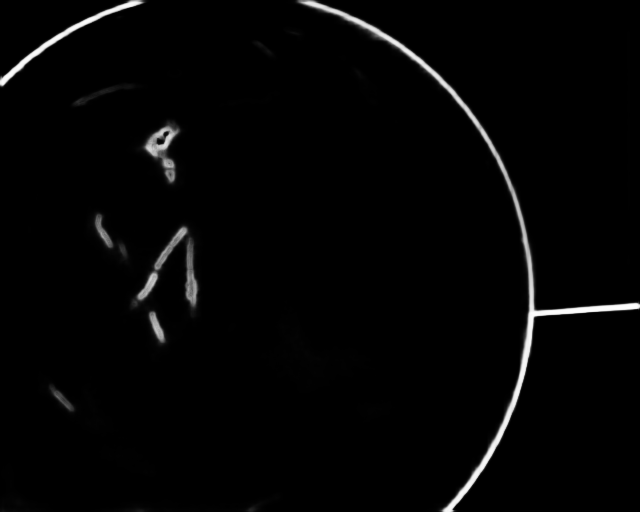}&
		\hspace{0.1cm}
		\includegraphics[width=0.235\linewidth]{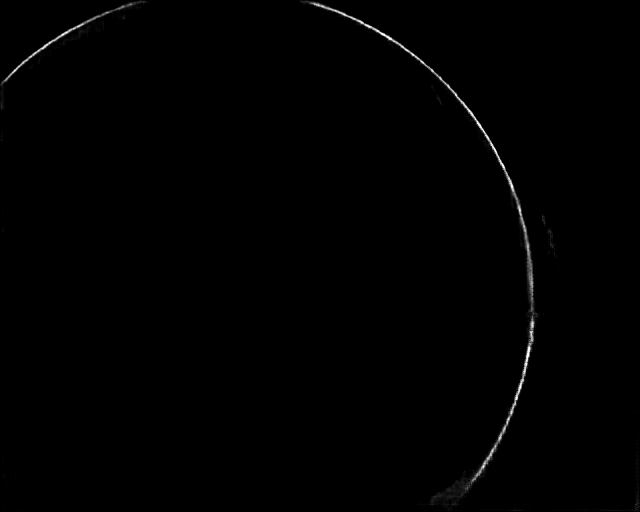}&
		\hspace{0.1cm}
		\includegraphics[width=0.235\linewidth]{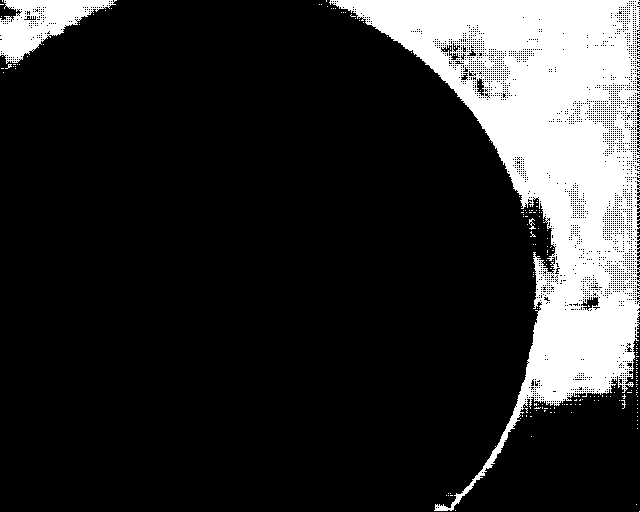}\\ 
		\includegraphics[width=0.235\linewidth]{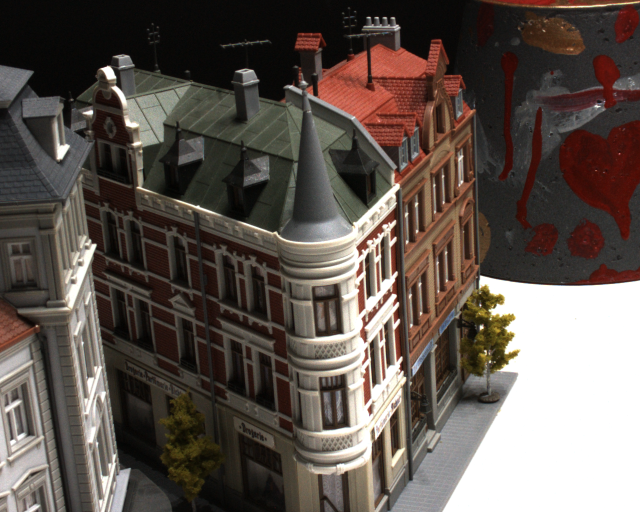}&
		\hspace{0.1cm} 
		\includegraphics[width=0.235\linewidth]{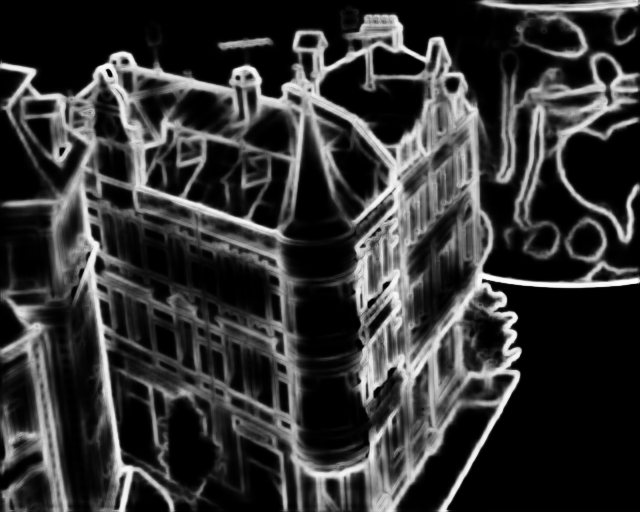}&
		\hspace{0.1cm} 
		\includegraphics[width=0.235\linewidth]{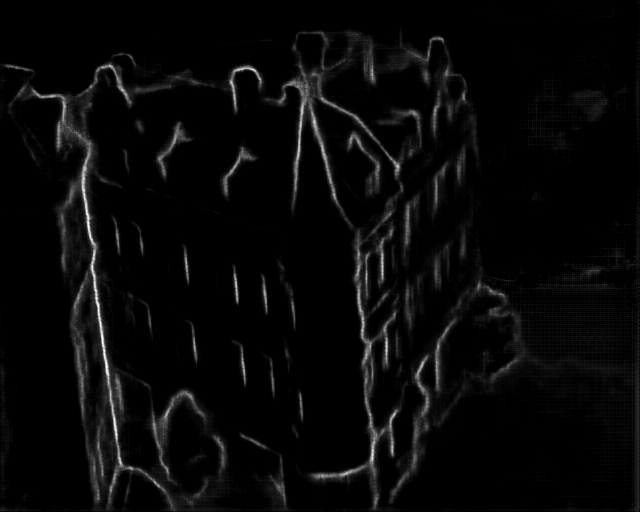}&
		\hspace{0.1cm} 
		\includegraphics[width=0.235\linewidth]{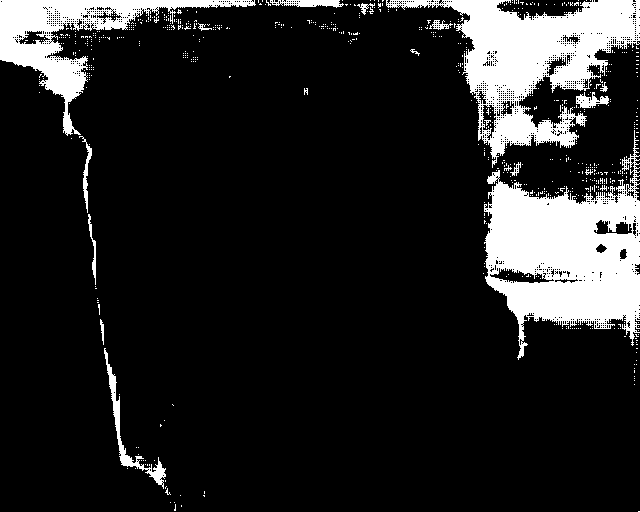}\\
		\includegraphics[width=0.235\linewidth]{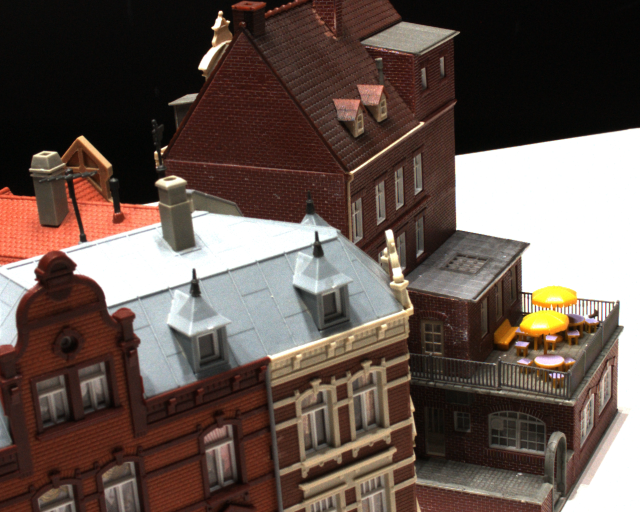}&
		\hspace{0.1cm} 
		\includegraphics[width=0.235\linewidth]{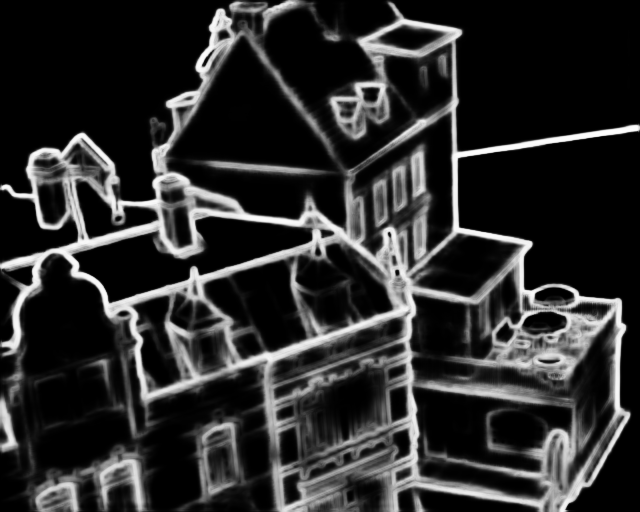}&
		\hspace{0.1cm} 
		\includegraphics[width=0.235\linewidth]{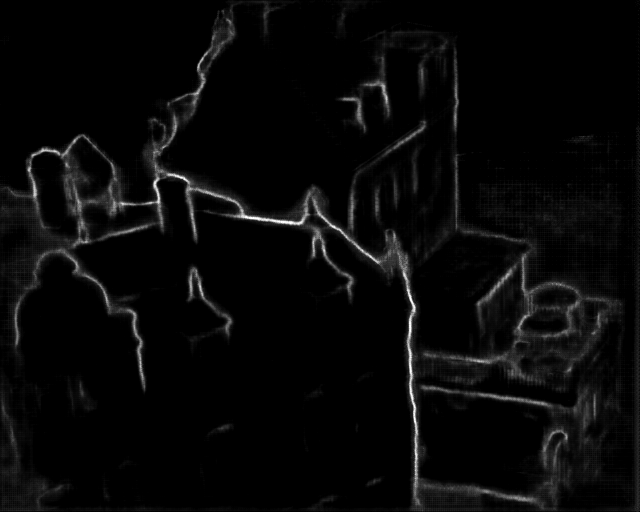}&
		\hspace{0.1cm} 
		\includegraphics[width=0.235\linewidth]{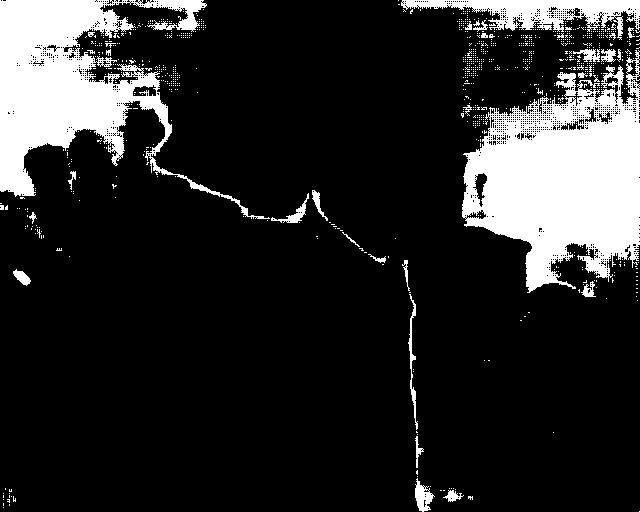}\\
		(a) & (b) & (c) & (d)
	\end{tabular}
	\caption{More edges maps (in addition to Fig. 4 of the paper) of a few randomly chosen examples. For each example, the images from left to right are:	(a) color image; (b) edge map predicted by HED~\cite{xie2015holistically}; (c) our learned edge map; (d) the $\alpha$ map.
		Our learned edge maps better capture the depth discontinuities, regardless of the photometric changes.
		It is also interesting to observe that our $\alpha$ maps distinguish between foreground and background. 
	}
	\label{fig:RGB_HED_EDGE_PI}
	
\end{figure}

%========================================================
\paragraph{Bimodal distribution.}
During development, we observed that Laplacian distribution had slightly better results than the Gaussian distribution on the depth map metrics on the validation set likely due to Laplacian having sharper peaks than the Gaussian. Both options will be provided in our source code. %===========================================================

\begin{figure*}[!t]
	\centering
	\begin{tabular}{c@{}c@{}c@{}c@{}}
		\includegraphics[width=0.235\linewidth]{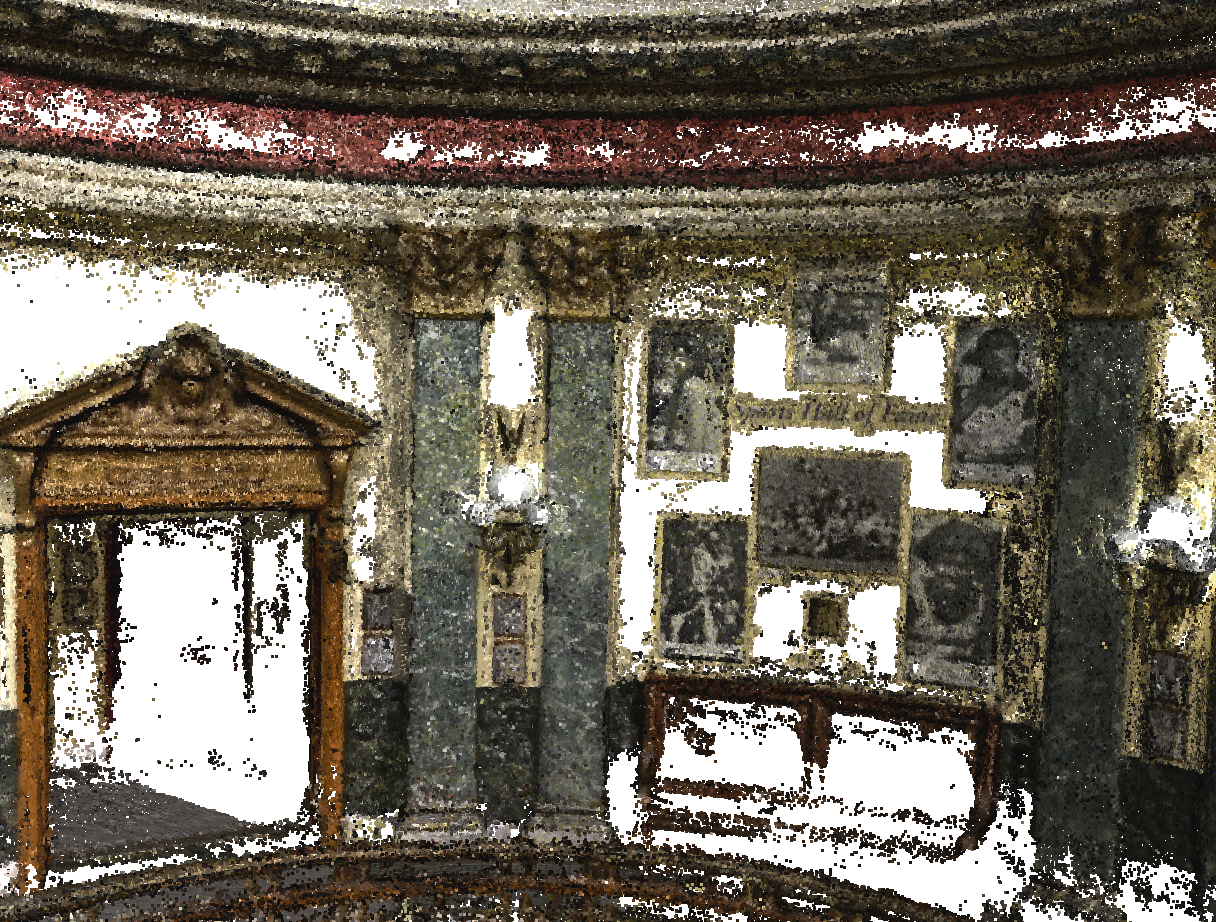} 
		\includegraphics[width=0.235\linewidth]{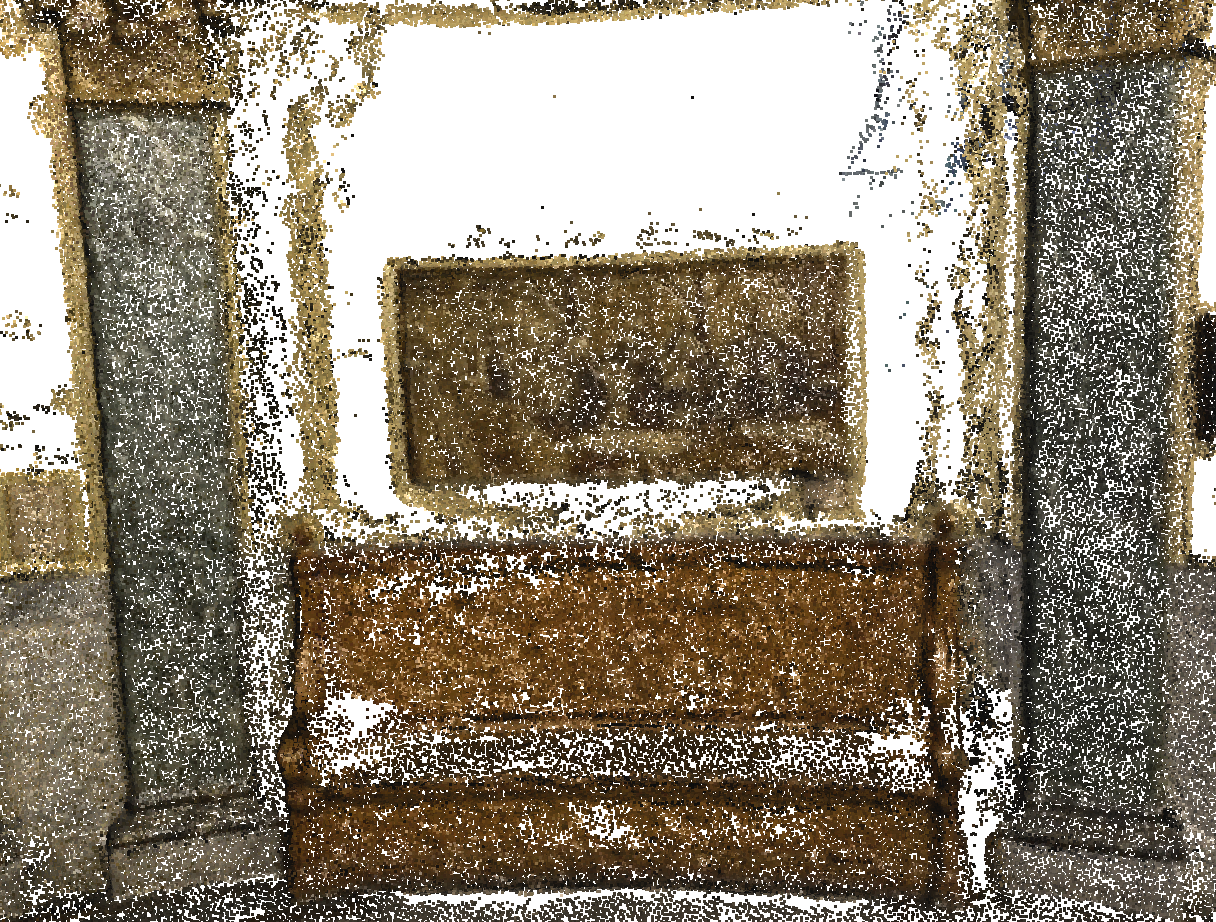} 
		\includegraphics[width=0.235\linewidth]{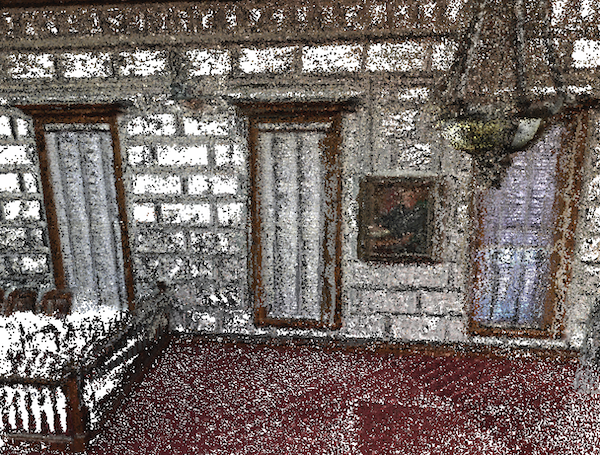} 
		\includegraphics[width=0.22\linewidth]{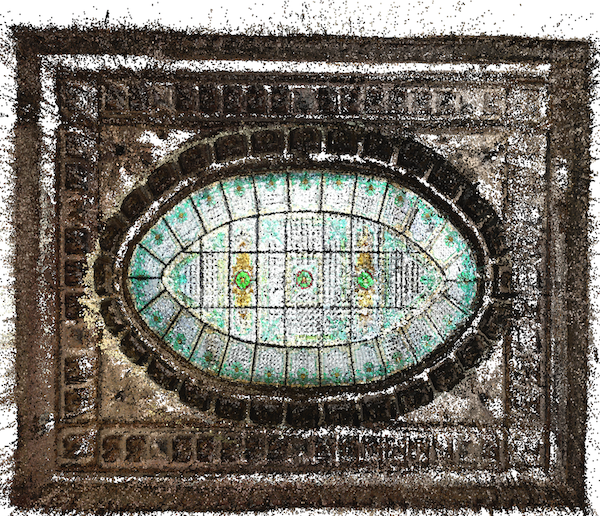}\\
		{COLMAP~\cite{schoenberger2016mvs}}
		\label{subfig:COLMAP}
	\end{tabular}
	\begin{tabular}{c@{}c@{}c@{}c@{}}	
		\includegraphics[width=0.235\linewidth]{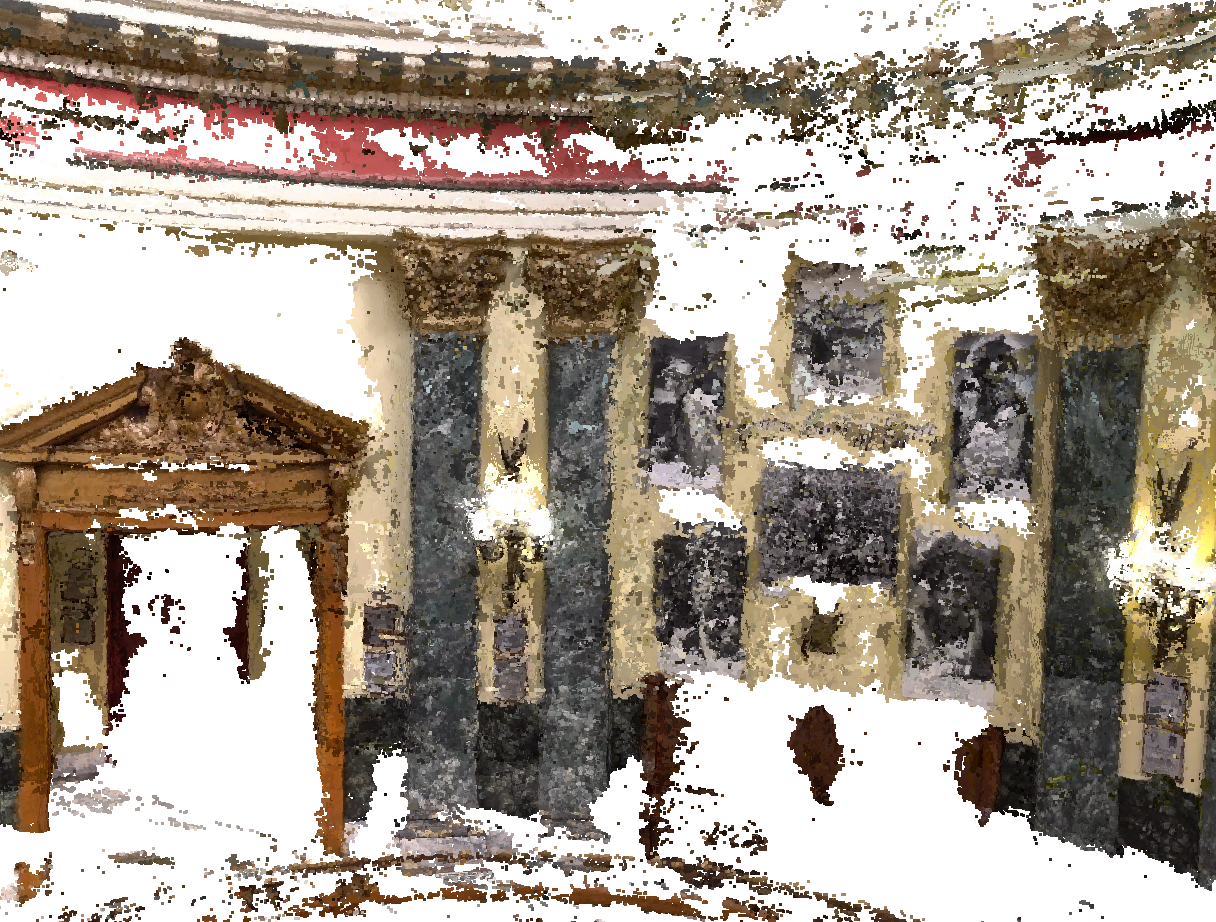} 
		\includegraphics[width=0.235\linewidth]{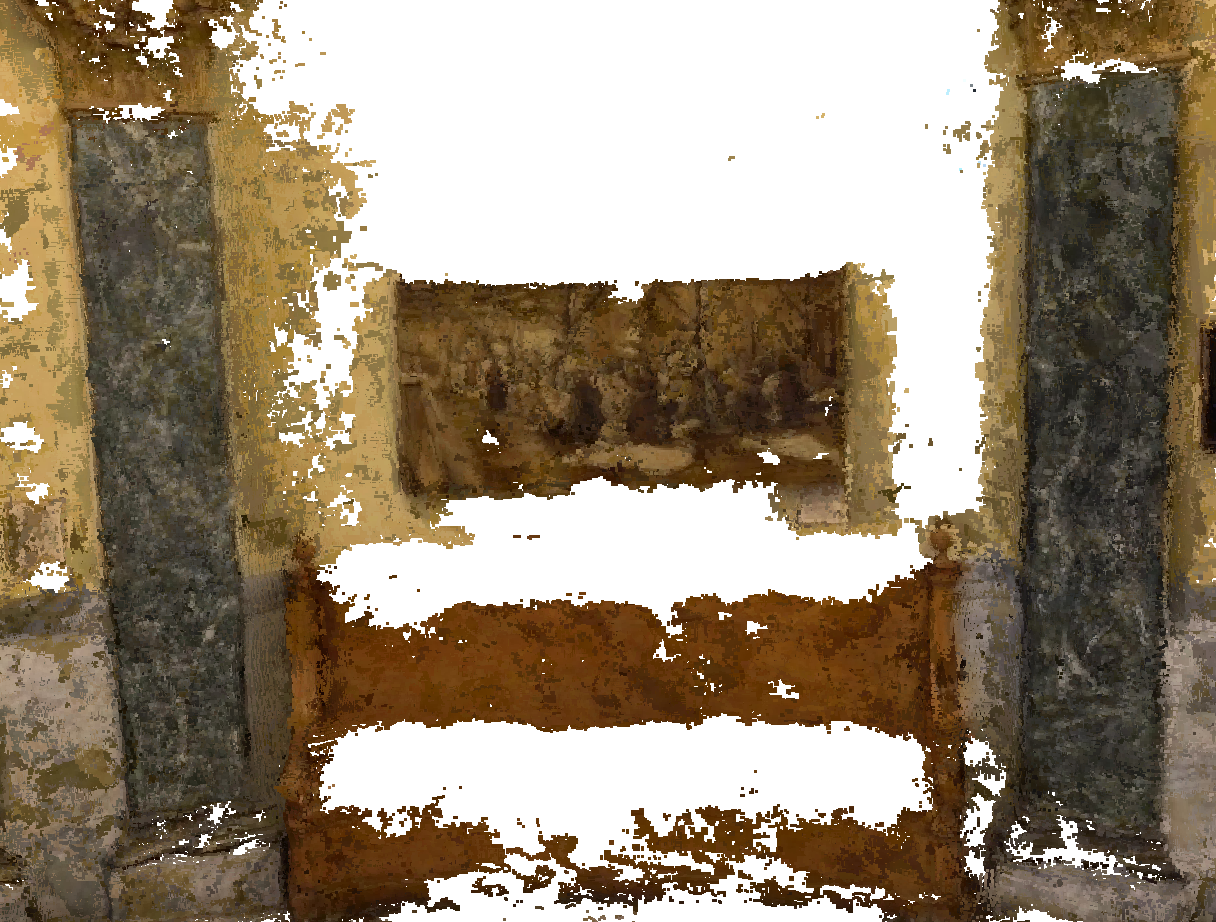} 
		\includegraphics[width=0.235\linewidth]{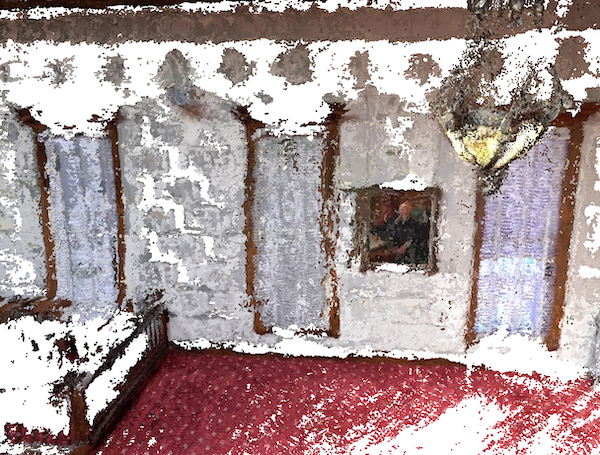} 
		\includegraphics[width=0.22\linewidth]{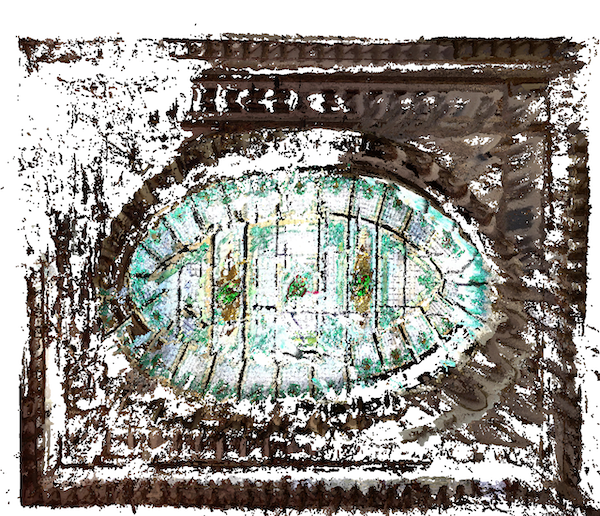}\\
		{PatchmatchNet~\cite{wang2020patchmatchnet}}
		\label{subfig:PatchmatchNet}
	\end{tabular}
	\begin{tabular}{c@{}c@{}c@{}c@{}}
		\includegraphics[width=0.235\linewidth]{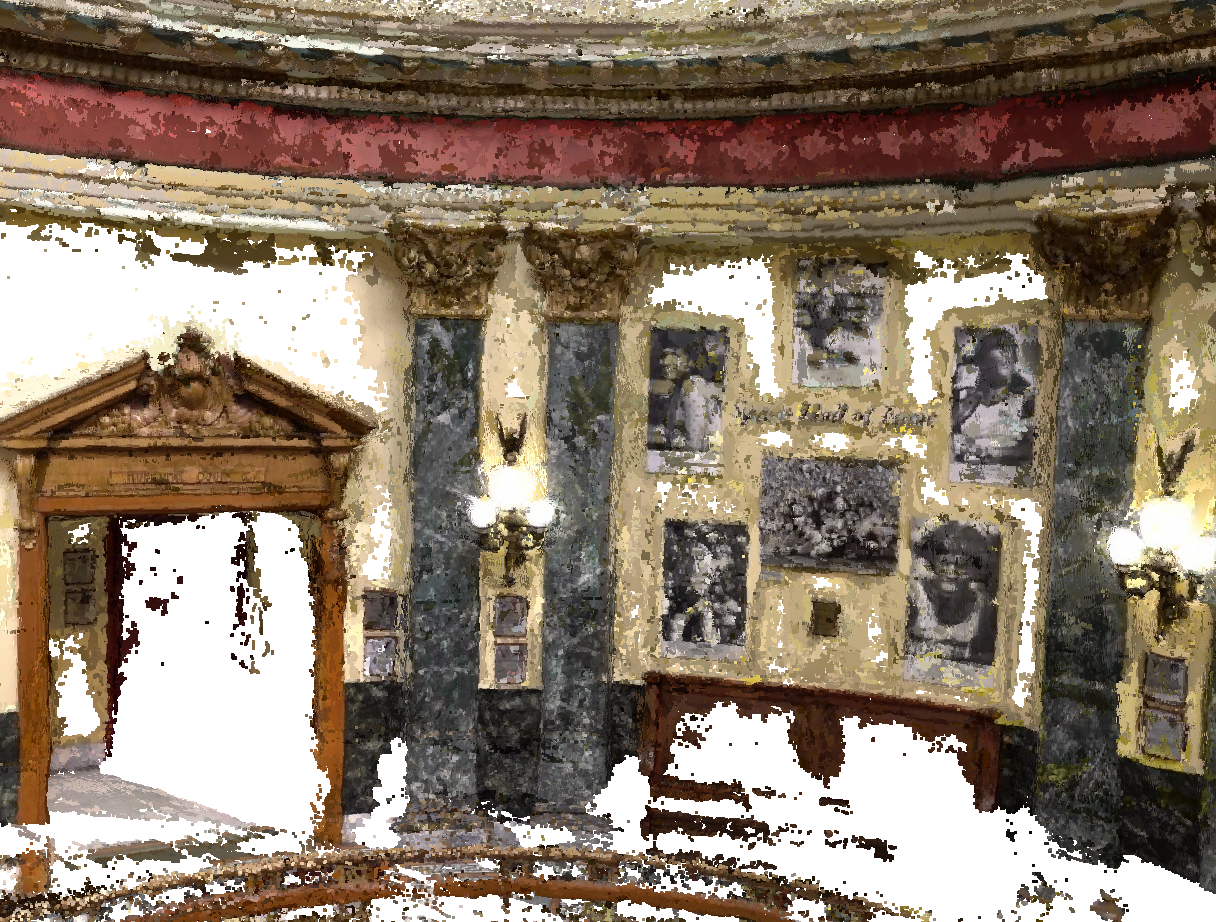} \hfill
		\includegraphics[width=0.235\linewidth]{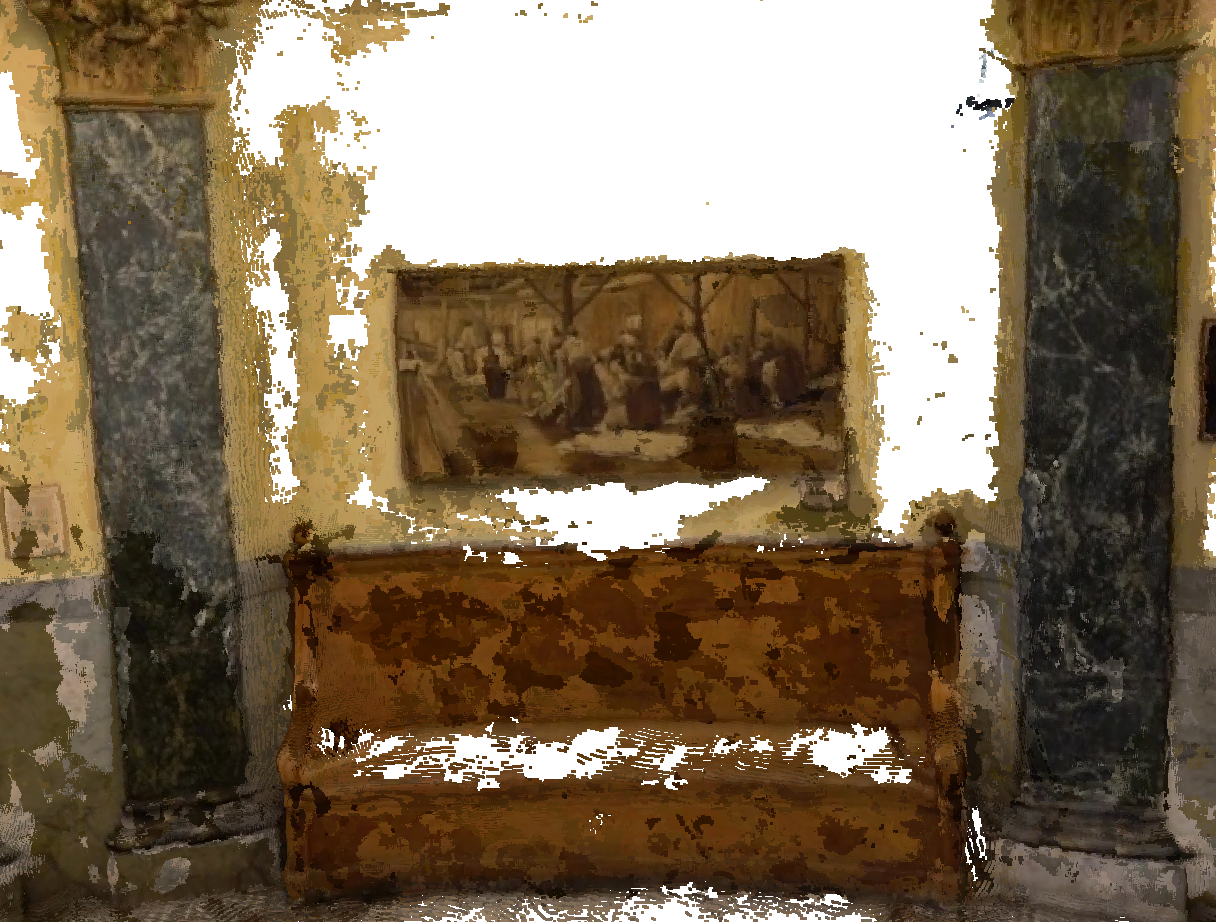} \hfill
		\includegraphics[width=0.235\linewidth]{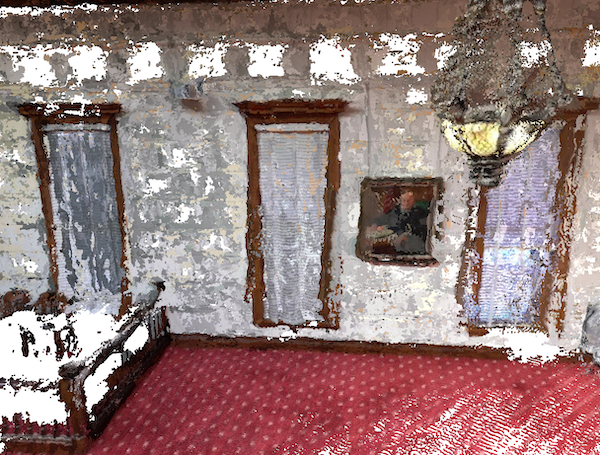}  \hfill
		\includegraphics[width=0.22\linewidth]{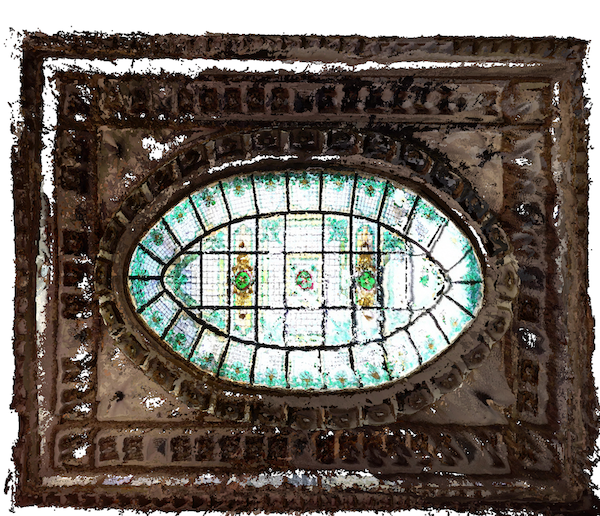}\\
		{Ours}
		\label{subfig:Ours}
	\end{tabular}
	\caption{\textbf{Comparisons with the state-of-the-art traditional photogrammetry-based MVS method COLMAP~\cite{schoenberger2016mvs} and learning-based MVS method PatchmatchNet~\cite{wang2020patchmatchnet}}. The results of four scenes are demonstrated in this figure. The last column visualizes the top of the \textit{courtroom} from the exterior. Please note that the lower part of the point cloud has been clipped to better reveal the completeness and accuracy of the ceiling.\\
		To have fair comparisons, we fed COLMAP with the ground-truth camera parameters. 
		Experiments show that the learning-based MVS method produces denser and more complete point clouds than the traditional photogrammetry-based method. However, the traditional photogrammetry-based method gives better accuracy, which is partially due to its sparsity. Among these methods, our results have the highest completeness and are cleaner. Compared to PatchmatchNet, our method is also superior in terms of reconstruction accuracy. Please refer to our paper for the quantitative results. More visual comparisons are available in the supplementary video.}
	\label{fig:compare}
	
\end{figure*}
