# Supplementary material for: DDL-MVS: Depth Discontinuity Learning for MVS Networks
Source: arXiv:2203.01391 source file (2023-06-12)
Supplement: Supplementary file 2 [file supp_comparison.tex]

\begin{figure}[htpb]
	\advance\leftskip-0.14cm
	\begin{tabular}{c@{}c@{}c@{}c}
		\includegraphics[width=0.23\linewidth]{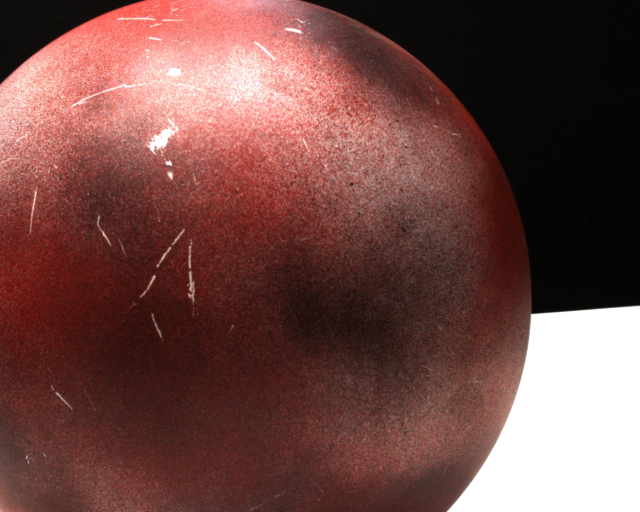}&
		\hspace{0.1cm}
		\includegraphics[width=0.23\linewidth]{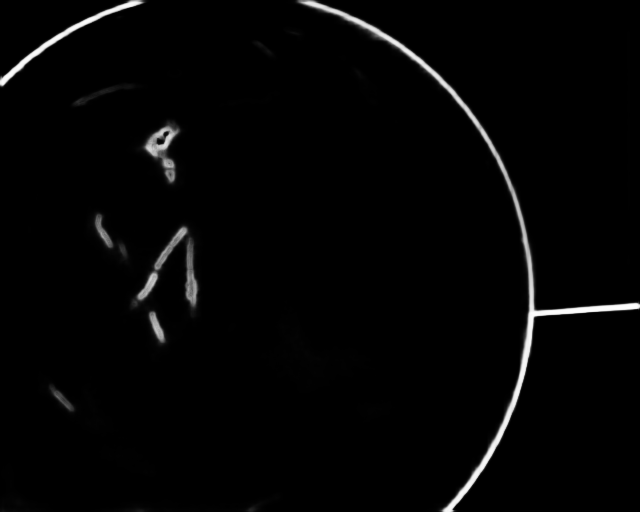}&
		\hspace{0.1cm}
		\includegraphics[width=0.23\linewidth]{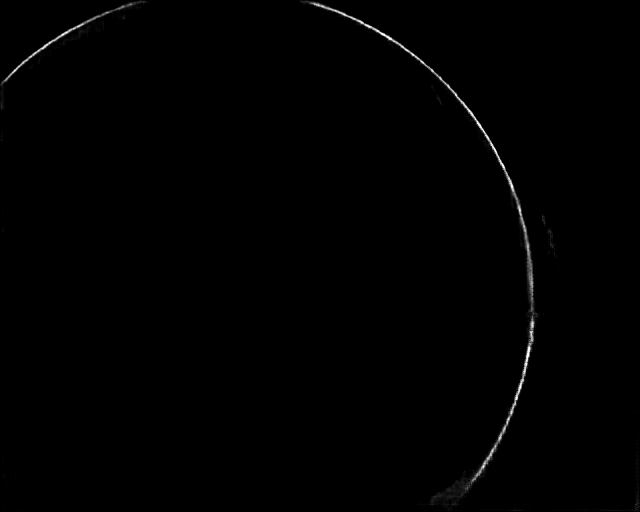}&
		\hspace{0.1cm}
		\includegraphics[width=0.23\linewidth]{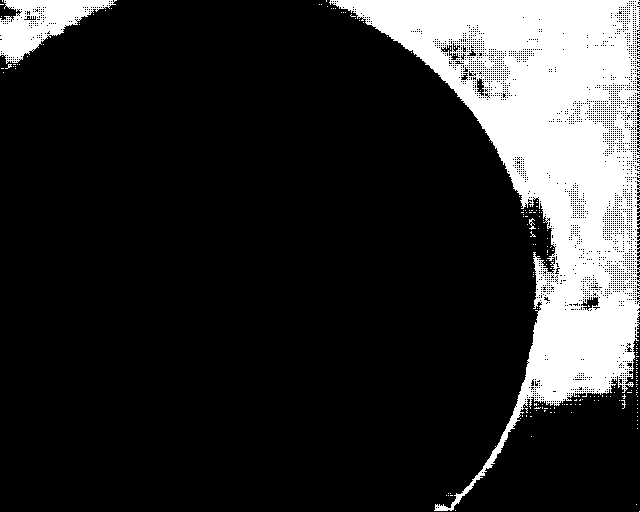}\\ 
		\includegraphics[width=0.23\linewidth]{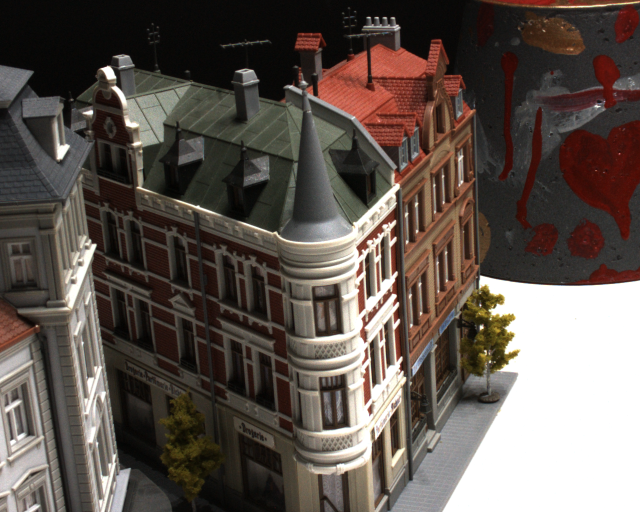}&
		\hspace{0.1cm} 
		\includegraphics[width=0.23\linewidth]{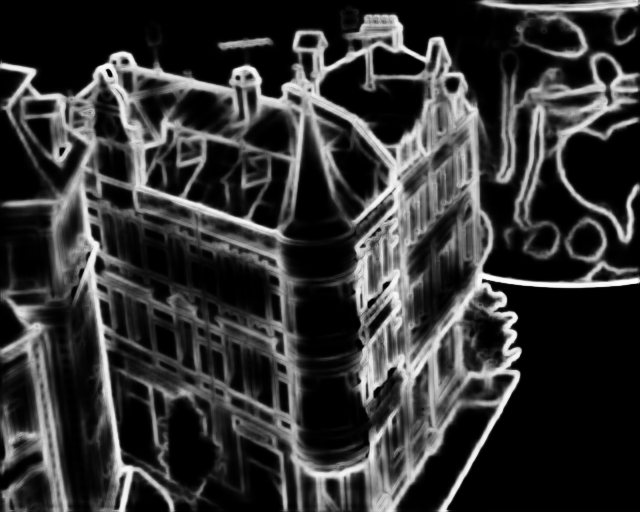}&
		\hspace{0.1cm} 
		\includegraphics[width=0.23\linewidth]{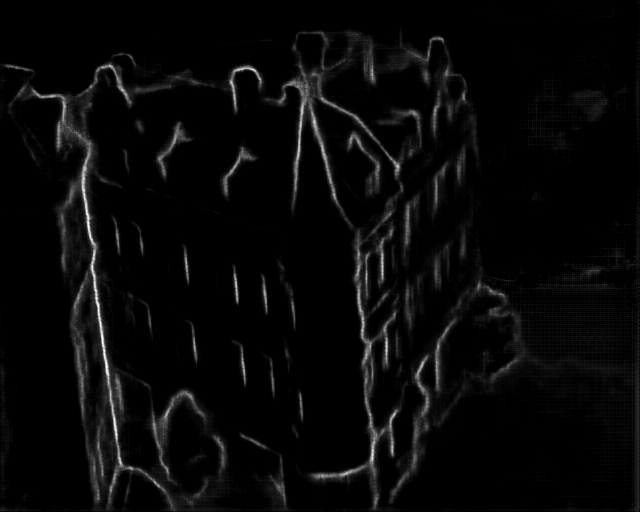}&
		\hspace{0.1cm} 
		\includegraphics[width=0.23\linewidth]{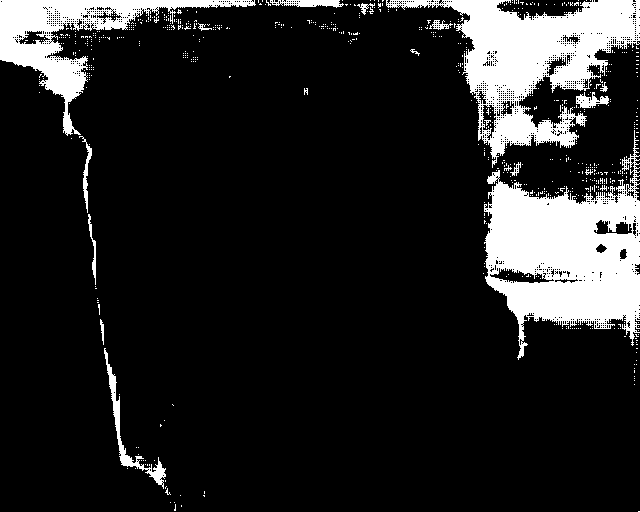}\\
		\includegraphics[width=0.23\linewidth]{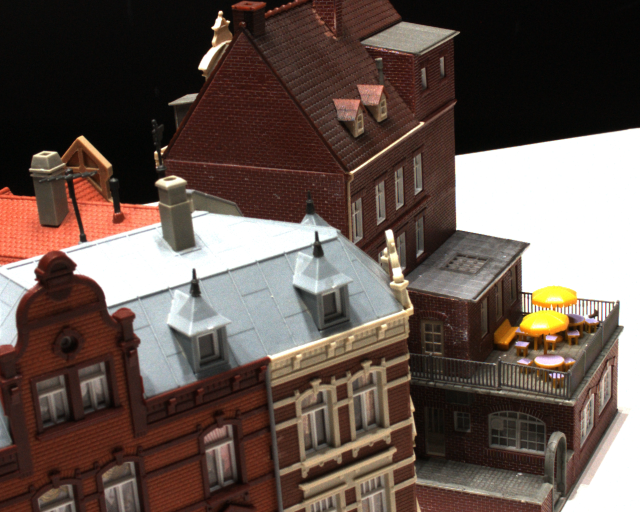}&
		\hspace{0.1cm} 
		\includegraphics[width=0.23\linewidth]{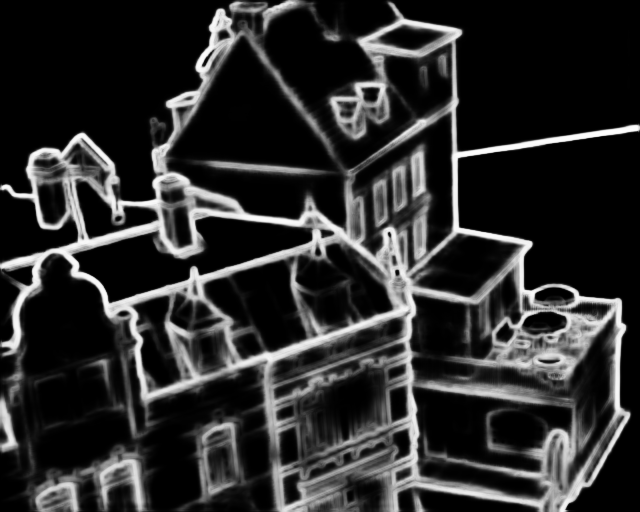}&
		\hspace{0.1cm} 
		\includegraphics[width=0.23\linewidth]{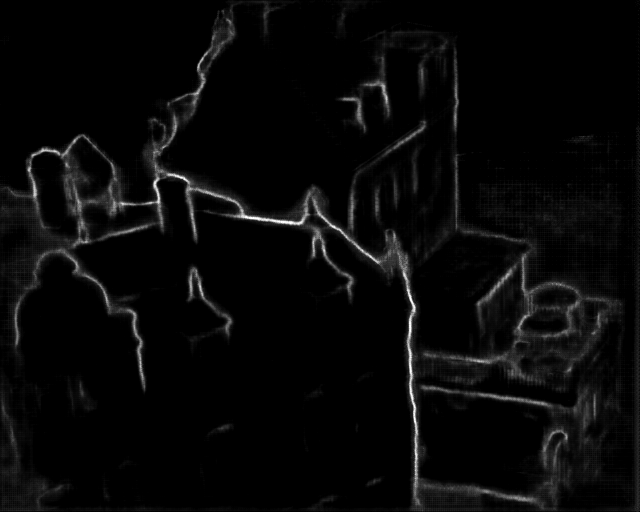}&
		\hspace{0.1cm} 
		\includegraphics[width=0.23\linewidth]{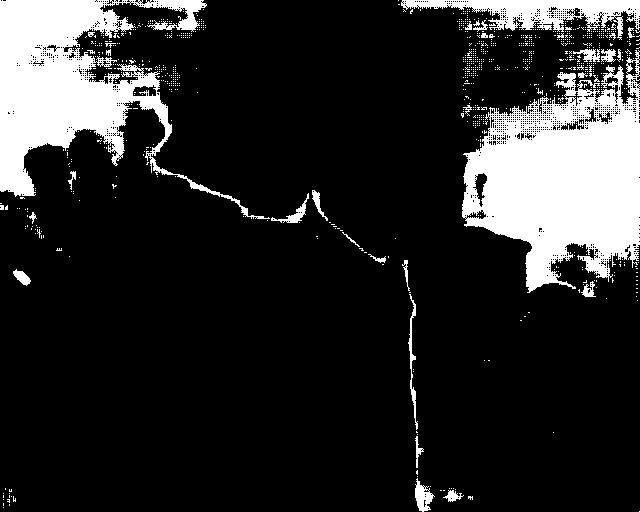}\\
		(a) & (b) & (c) & (d)
	\end{tabular}
	\caption{More edges maps (in addition to Fig. 4 of the paper) of a few randomly chosen examples. For each example, the images from left to right are:	(a) color image; (b) edge map predicted by HED~\cite{xie2015holistically}; (c) our learned edge map; (d) the $\alpha$ map.
		Our learned edge maps better capture the depth discontinuities, regardless of the photometric changes.
		It is also interesting to observe that our $\alpha$ maps distinguish between foreground and background. 
	}
	\label{fig:RGB_HED_EDGE_PI}
	
\end{figure}

\begin{figure*}[!ht]
	\centering
	\begin{tabular}{c@{}c@{}c@{}c@{}}
		\includegraphics[width=0.235\linewidth]{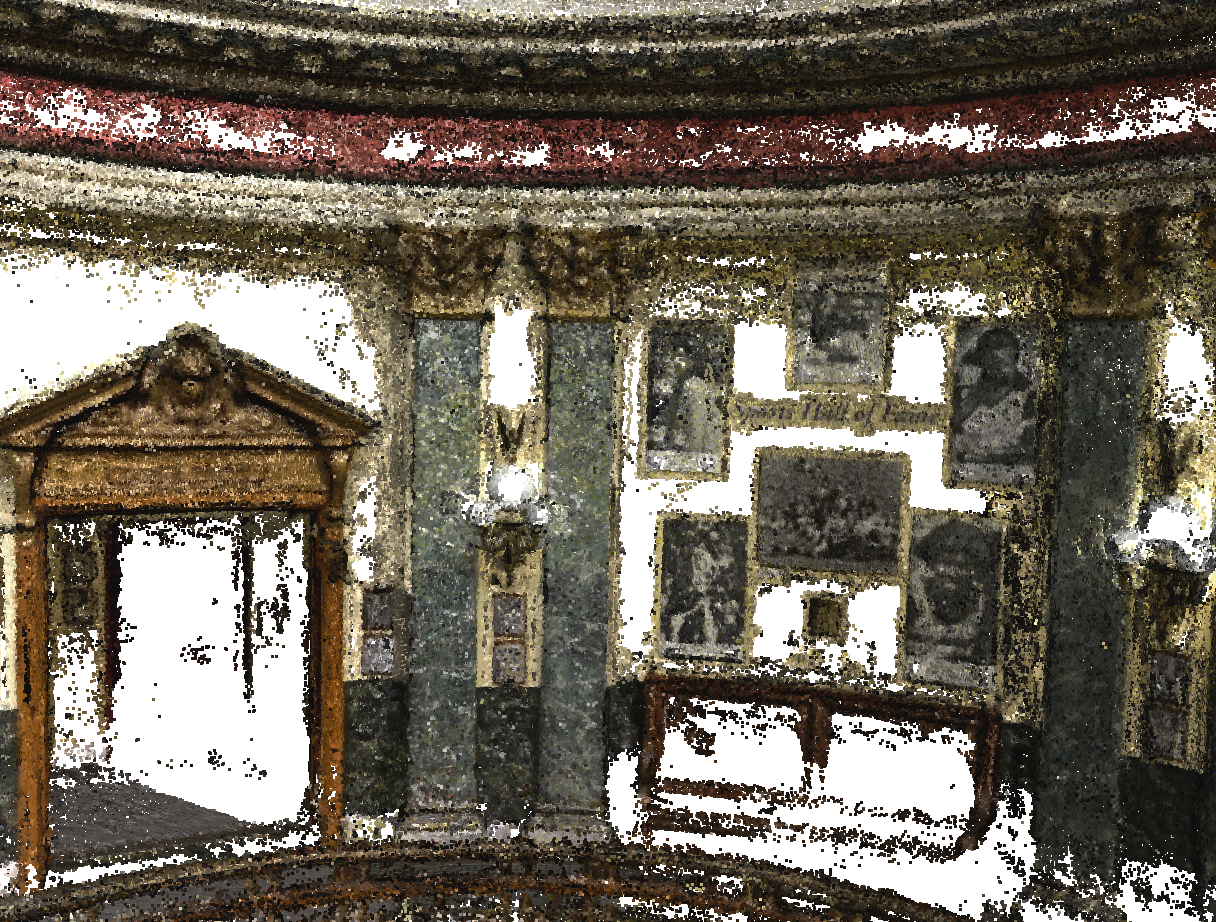} 
		\includegraphics[width=0.235\linewidth]{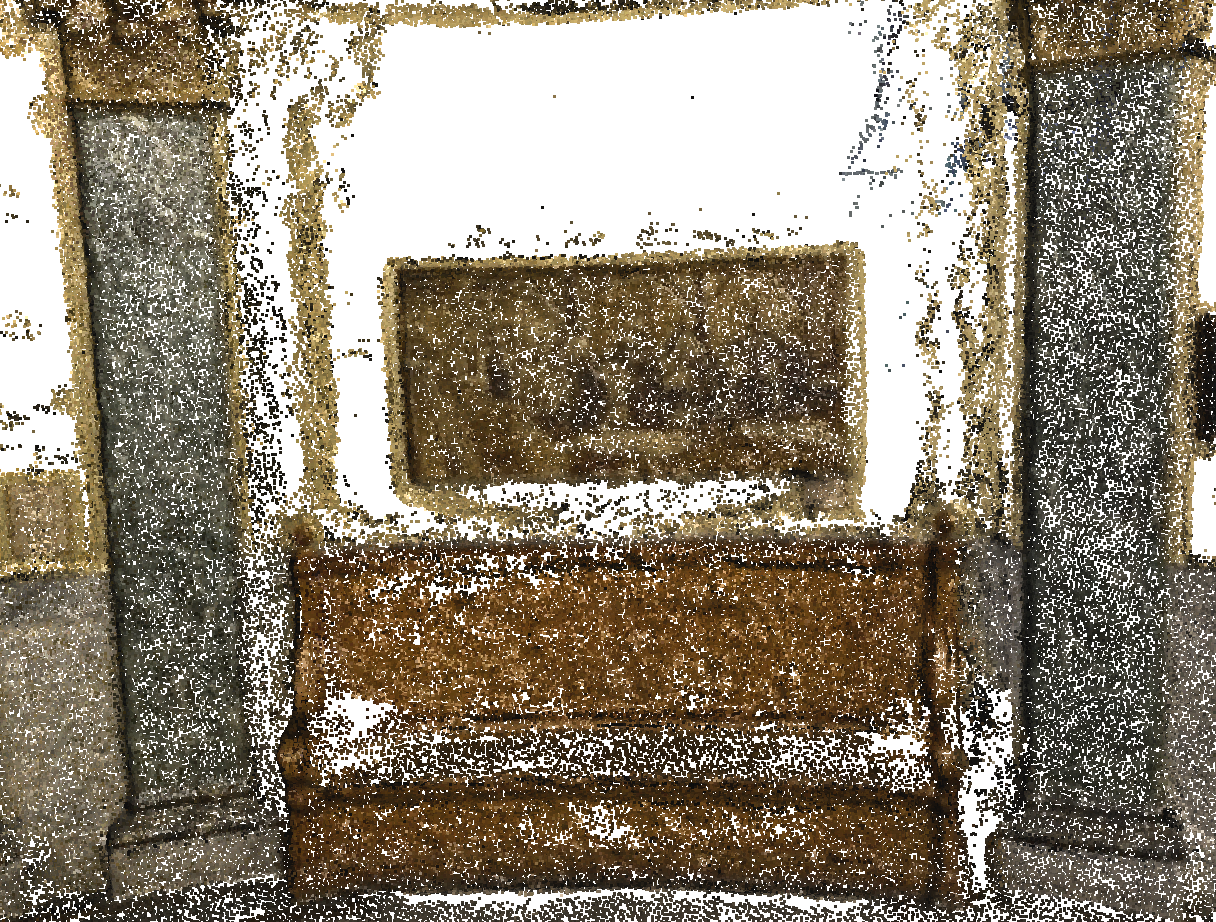} 
		\includegraphics[width=0.235\linewidth]{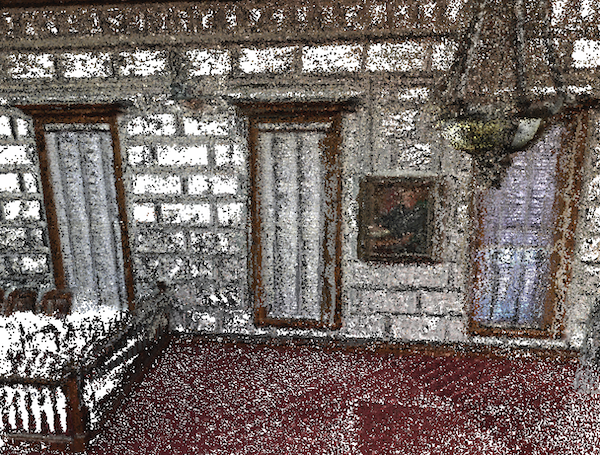} 
		\includegraphics[width=0.22\linewidth]{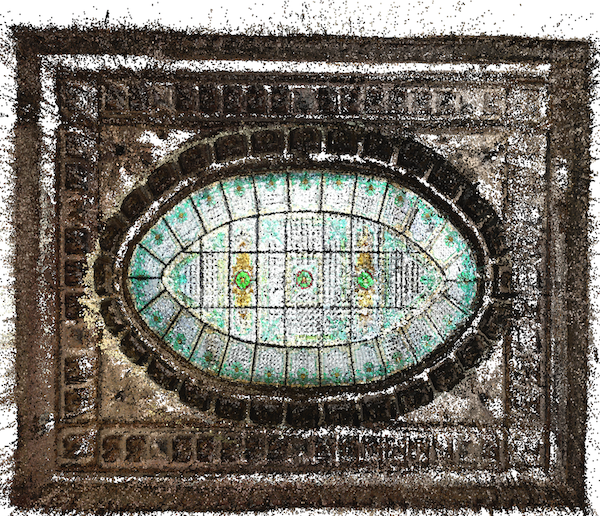}\\
		{COLMAP~\cite{schoenberger2016mvs}}
		\label{subfig:COLMAP}
	\end{tabular}
	\begin{tabular}{c@{}c@{}c@{}c@{}}	
		\includegraphics[width=0.235\linewidth]{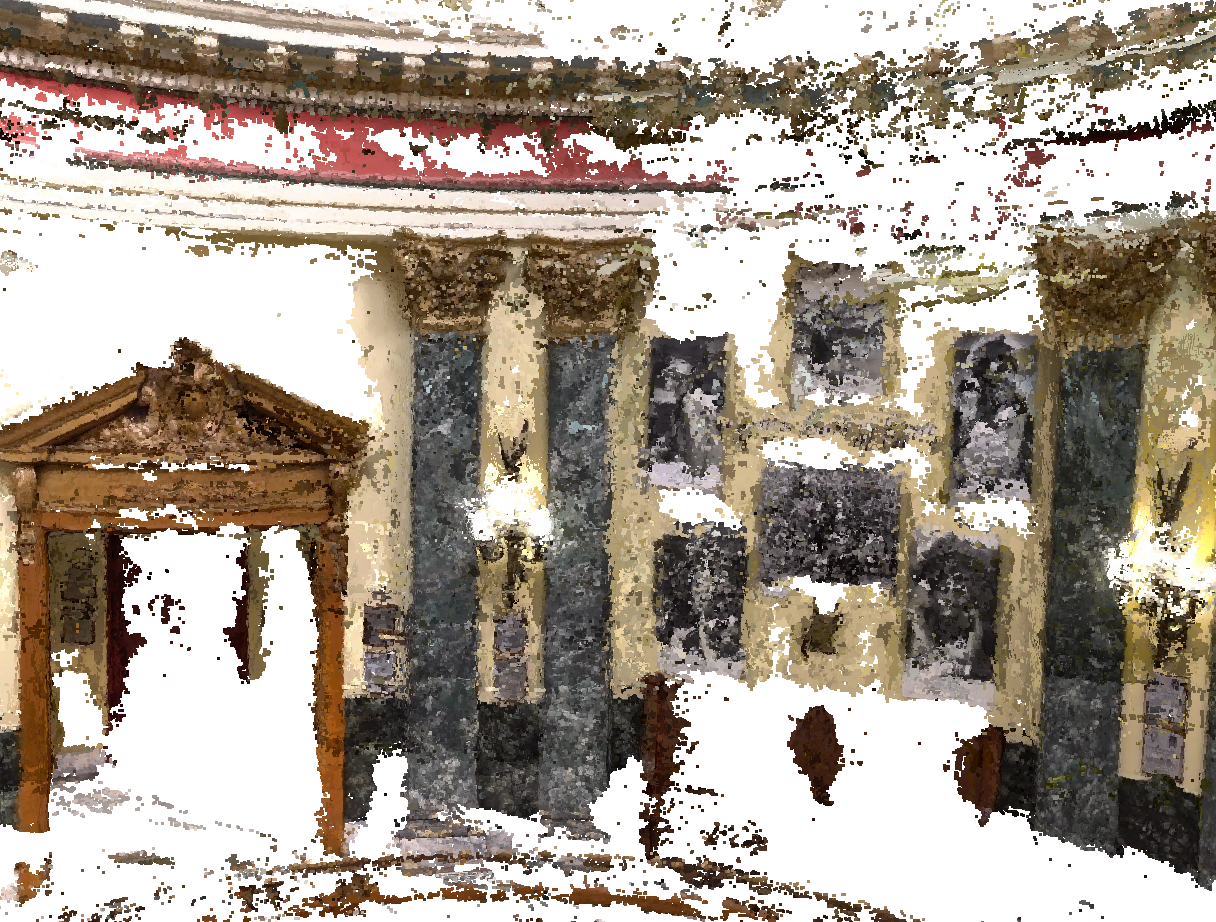} 
		\includegraphics[width=0.235\linewidth]{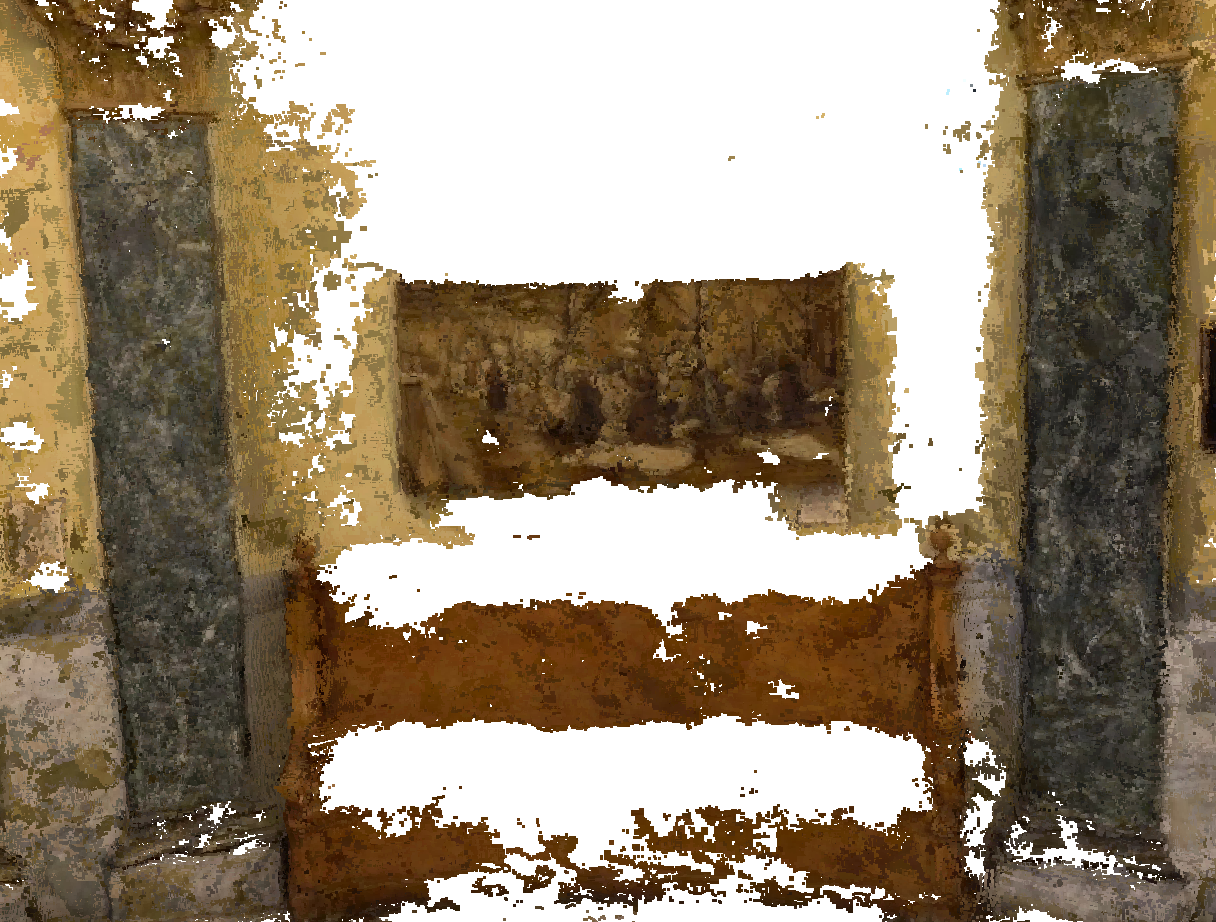} 
		\includegraphics[width=0.235\linewidth]{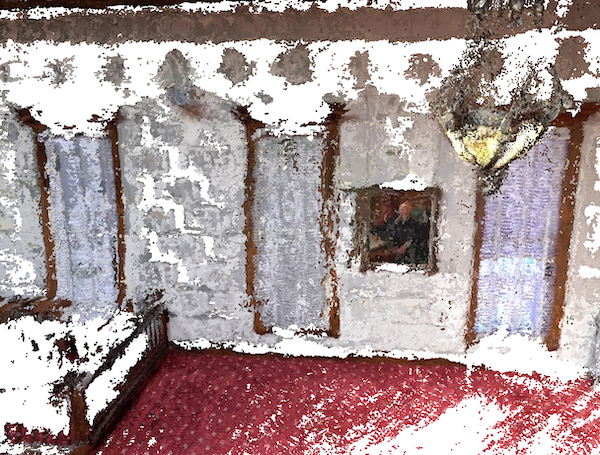} 
		\includegraphics[width=0.22\linewidth]{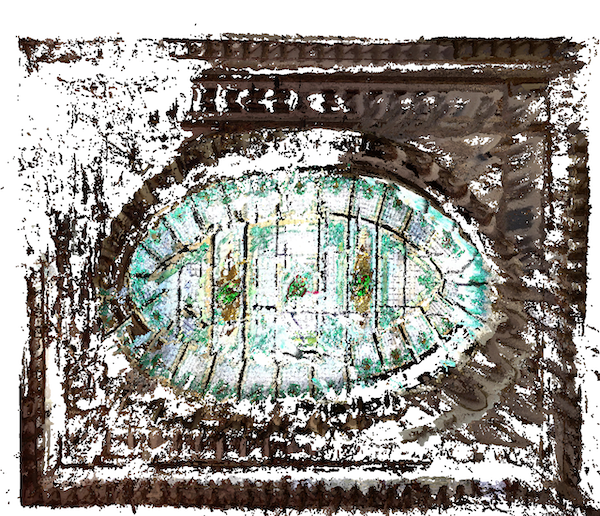}\\
		{PatchmatchNet~\cite{wang2020patchmatchnet}}
		\label{subfig:PatchmatchNet}
	\end{tabular}
	\begin{tabular}{c@{}c@{}c@{}c@{}}
		\includegraphics[width=0.235\linewidth]{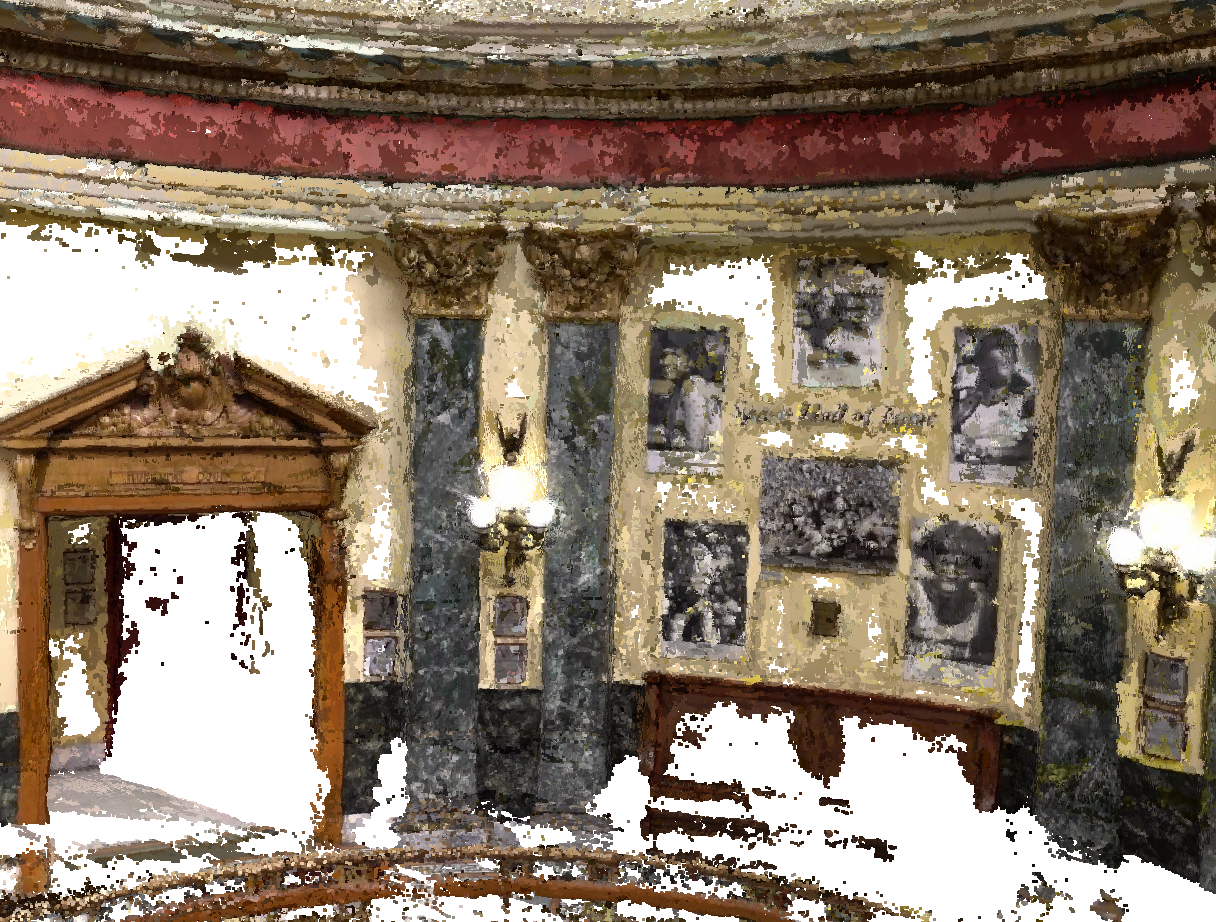} \hfill
		\includegraphics[width=0.235\linewidth]{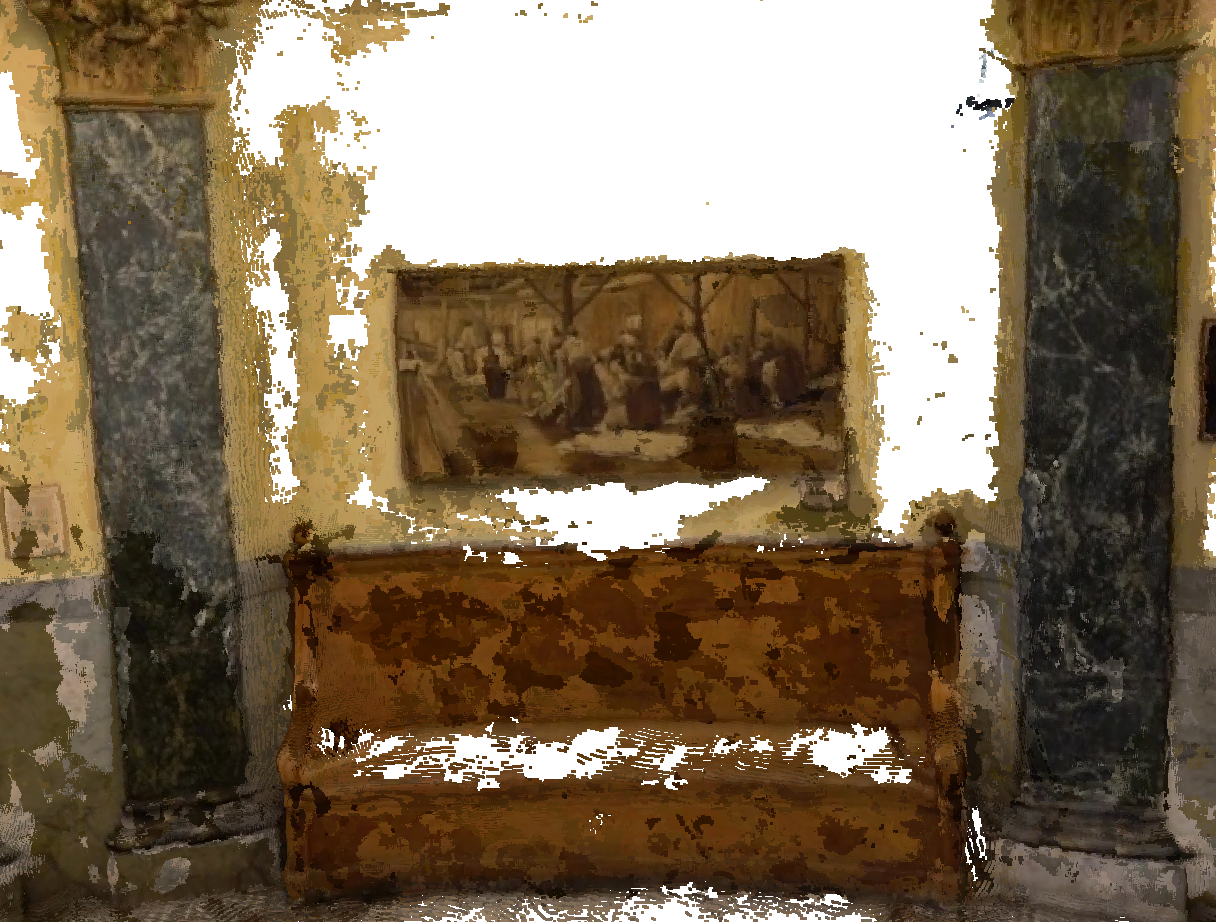} \hfill
		\includegraphics[width=0.235\linewidth]{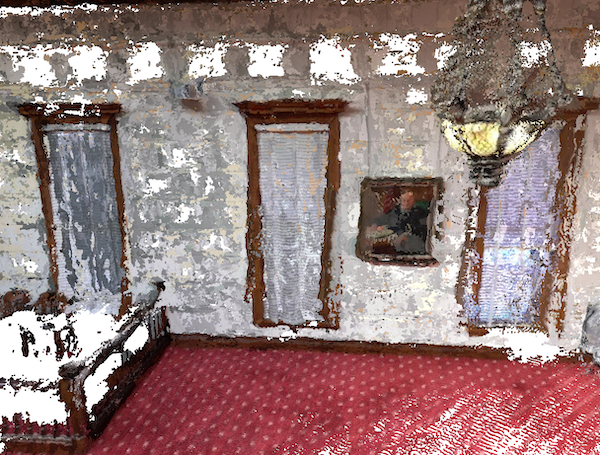}  \hfill
		\includegraphics[width=0.22\linewidth]{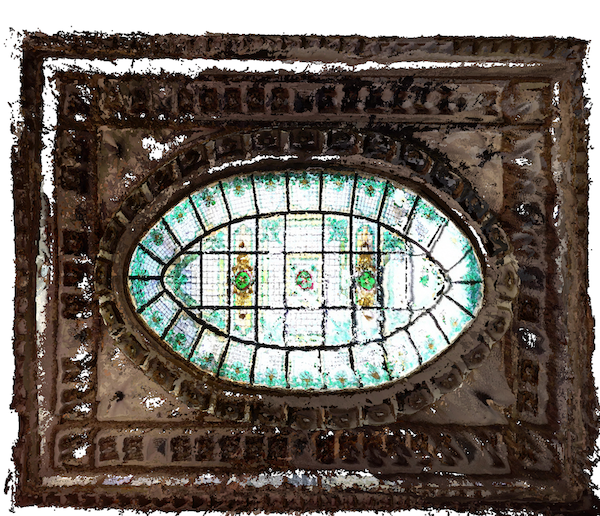}\\
		{Ours}
		\label{subfig:Ours}
	\end{tabular}
	\caption{\textbf{Comparisons with the state-of-the-art traditional photogrammetry-based MVS method COLMAP~\cite{schoenberger2016mvs} and learning-based MVS method PatchmatchNet~\cite{wang2020patchmatchnet}}. The results of four scenes are demonstrated in this figure. The last column visualizes the top of the \textit{courtroom} from the exterior. Please note that the lower part of the point cloud has been clipped to better reveal the completeness and accuracy of the ceiling.\\
		To have fair comparisons, we fed COLMAP with the ground-truth camera parameters. 
		Experiments show that the learning-based MVS method produces denser and more complete point clouds than the traditional photogrammetry-based method. However, the traditional photogrammetry-based method gives better accuracy, which is partially due to its sparsity. Among these methods, our results have the highest completeness and are cleaner. Compared to PatchmatchNet, our method is also superior in terms of reconstruction accuracy. Please refer to our paper for the quantitative results. More visual comparisons are available in the supplementary video.}
	\label{fig:compare}
	
\end{figure*}
